# Supplementary material for: Unsupervised Co-part Segmentation through Assembly
Source: arXiv:2106.05897 source file (2021-06-10)
Supplement: Supplementary file 5 [file rebuttal.tex]

%\documentclass{article}

% Use the following line for the initial blind version submitted for review:
%\usepackage{icml2021_author_response}
%\usepackage{geometry}
%\geometry{left=0.5in,right=0.5in,top=0.5in,bottom=0.5in}

%\usepackage{xcolor}
%\input{content/x_preamble}

%\usepackage{sectsty}
%\sectionfont{\normalsize}

%\usepackage{titlesec}

%\titleformat{\section}{\normalfont\normalsize\bfseries}{$\bullet$}{1em}{}
%\titlespacing{\section}{0pt}{1ex}{1ex}



%\usepackage{multirow}
%\usepackage{cases, enumerate}

%\begin{document}
\onecolumn
%\date{}
%\title{Rebuttal}
%\author{Paper ID 2352}
%\maketitle
%\pagestyle{empty}

\section{\blue{**Rebuttal is in the next page}}

\section{Experiments}
\begin{itemize}
    \item generalization: (finished)
    \begin{itemize}
        \item apply TaiChi model to Yoga
        \item apply Yoga model to TaiChi
        \item find a video on Youtube and apply TaiChi/Yoga to it
        \item find a video on Youtube and apply Face model to it
        
        \item (optional) train model with all the videos
    \end{itemize}
    
    \item moving background - training on DAVIS dataset
    \begin{itemize}
        \item train on single video
        \item train on several videos and show generalization
    \end{itemize}
    
    \item multiple object - training on DAVIS dataset/ other videos
    \begin{itemize}
        \item try our model on videos with mulitple characters/faces 
        \item train on single video with two characters (DAVIS or other video)
        \item or train on single video with some other objects
    \end{itemize}
    
    \item ablation study of Transformation loss on Face dataset
    
    \item apply erosion to Motion Co-Part result, possibly showing that the segments becomes apart, or showing that we cannot make the mask consistently tightly.
    
    \item ablation study of K
    
    \item check the order of magnitude of every loss term 
    (around 0.1)
    
\end{itemize}



%%%%%%%%%%%%%%%%%%%%%%%%%%%%%%%%%%%%%%%%%%%%%%%%%%%%%%%%%%%%%%%%%%
\clearpage
%%%%%%%%%%%%%%%%%%%%%%%%%%%%%%%%%%%%%%%%%%%%%%%%%%%%%%%%%%%%%%%%%%

We thank all the reviewers for taking the time to read our submission and provide positive and constructive comments. Below we first address common concerns raised in the reviews then answer each individual questions.

\section{generalization of the method, training on single/multiple videos (R1, R6)}
\input{figures/rebuttal_view}

Our model can be trained using either a single video or a collection of videos. We only assume that the two images in an image pair have similar appearance, but these image pairs can be collected from multiple videos of different subjects. We have shown in the paper both the results trained with \textbf{single-video settings} (hand, quadruped, and robot arm) and the results with \textbf{multiple-video settings} (Tai-Chi-HD, VoxCeleb, and Exercise datasets).

Models trained with multiple videos can generalize well to images of the same category but with difference appearance. For example, the images shown in Fig.~5 and Fig.~6 of our paper are from the test set of Tai-Chi-HD and VoxCeleb datasets respectively, which were not seen by the networks during training. Without further training, the models trained on these two datasets can be applied to videos downloaded from YouTube, as shown in Fig.~\ref{fig:rebuttal_generalization} above.

\section{trivial solutions (R3, R5), images pairs (R1), part correspondence (R1), optimum $K$ (R5)}
During training, we require the network to reconstruct source image and target image as accurate as possible, the trivial solutions could not get the accurate target image. And if we do not use images pairs, it maybe get trivial solution.

Our method is unsupervised, the segmentation does not necessarily correspond to the human annotated object parts. Like previous works,  we manually select our parts to correspond the ground-truth in Exercise dataset. In Tai-Chi-HD and VoxCeleb datasets, we use two metrics without correspondence.

In experiment, we set $K$ same to previous work to compare. In practice, the $K$ is not sensitive to the result when $K$ is big enough. For hand, quadruped, and robot arm, we set the $K$ is $16$, it works well.

\section{failure cases (R3)}
Our method can not distinguish left and right of human. When person cross  legs or arms, the correspondence is  wrong. 
\section{loss weights (R3), background loss (R5), transformation loss (R5)}
For loss weights setting, we set order of magnitude of every loss term (except reconstruction loss) to be same (0.1) based on experience. 
transformation loss does not have clear effect on VoxCeleb. 
\blue{Background is same to  trivial solutions}

\section{erosion (R1)}

\section{moving background, DAVIS dataset (R1)}
In our method, we assume that the background is static.  In experiment, the slight translation can be handle.  In Tai-Chi-HD and  VoxCeleb datasets, the background is not totally static. But in DAVIS dataset, the background has more change, our method is not suitable for it without supervision.  
\section{multiple objects (R1)}
In our setting, we do not limit the number of objects in the video, it can use the same way to train. 
%\end{document}
